# Supplementary material for: Analysis of the Optimization Landscapes for Overcomplete Representation Learning
Source: arXiv:1912.02427 source file (2019-12-10)
Supplement: Supplementary file 1 [file appendix.tex]

%xxxxxxxxxxxxxxxxx

%\section{Basic Tools}

%\input{sections/appendix/tools}
